# Supplementary material for: Rearranged Stochastic Heat Equation: Ergodicity and Related Gradient Descent on ${\mathcal P}({\mathbb R})$
Source: arXiv:2403.16140 source file (2024-06-10)
Supplement: Supplementary file 1 [file appendix.tex]

%!TEX root = ../main_rshe_ergodic.tex

We give a proof of \eqref{eq lipShiftIneq}

\begin{proposition}\label{prop proofOfLipShiftIneq} For

$T^2 > (2T+1)R^2$, $u$ and $v \in U^2(\bS)$ such that $\| u \|_2, \| v \|_2\leq R$ and any finite $M$, the following inequality holds $\bP$ almost surely:

\begin{equation} 
	\begin{split}
		&  \bigl\lVert X_t^{u_t^{*,M}(z)}-X^{u^{*,M}}_t  \bigr\rVert_2^2 +2\int_0^t  \bigl\lVert   \nabla_x \bigl(X_s^{u_s^{*,M}(z)}-X^{u^{*,M}}_s \bigr)
		\bigr\rVert_2^2 \d s 
		\\
		&\leq   \bigl\lVert  X_0^{u_0^{*,M}(z)}-X^{u^{*,M}}_0 \bigr\rVert_2^2 +\int_0^t \bigl\lVert  X_s^{u_s^{*,M}(z)}-X^{u^{*,M}}_s \bigr\rVert_2^2 \d s 
		\\
&\hspace{15pt}		+ \tfrac{1}{T^2} \sum_{m\geq 0}\int_0^t |  D_M \bigl\langle  X^{u^{*,M}_t(z)}_s ,e_m\bigr\rangle \cdot {z^M} |^2   \d s,
	\end{split}
\end{equation}
where $z:=v-u$.
\end{proposition}

Naturally, the proof will use the dynamics of the shifted process and its tilted reflection process. These have already been identified in Propositions 5.7 and 5.8 in \cite{delarueHammersley2022rshe} and are recalled presently.
For $z \in  {E^M}$, $\bP$ almost surely, 
for Lebesgue almost every $u \in E^M$, for any $h \in H^2_{\rm sym}({\mathbb S})$,  
\begin{equation}
	\label{eq shiftedDynamics}
	\begin{split}
		\bigl\langle    X^{u_t^{*,M}(z) }_t , h  \bigr\rangle    	=  &   \bigl\langle    X^{(u+z)^{*,M}}_0 , h \bigr\rangle + 
		\int_0^t \bigl\langle    X^{u^{*,M}_s(z)}_s  ,\Delta_x h \bigr\rangle   \d s 
		+  \int_0^t   \d \bigl\langle \tilde{\eta}^{\textcolor{black}{u,(z,1)}}_s, h \bigr\rangle   
		\\
		&+ \int_0^t \d \langle  {W}_s  ,h\rangle   -    \tfrac{1}{T}  \int_0^t \partial_y \bigl\langle  X^{u^{*,M}_s(z)}_s ,h\bigr\rangle \cdot z   \,   \d s, 
	\end{split} 
\end{equation}
where $\tilde \eta^{u,(z,1)}$ is the \emph{tilted} reflection process satisfying the requisite conditions (2. and 4.) of Definition \ref{def:existence} (under $\bQ$, {see \eqref{eq qTau}}). 

\begin{proof}
One begins by applying the standard Itô formula to $\langle X_t^{u_t^{*,M}(z)}-X^{u^{*,M}}_t,e^{\varepsilon\Delta}e_m \rangle^2$ and sums over $m$. This leads to the following (having denoted $e^\varepsilon_m:=e^{\varepsilon\Delta}e_m$),

\begin{align}
\nonumber		\d \bigl\lVert e^{\varepsilon\Delta}(X_t^{u_t^{*,M}(z)}-X^{u^{*,M}}_t  )\bigr\rVert_2^2 = & 2\sum_{m\geq 0}\langle X_t^{u_t^{*,M}(z)}-X^{u^{*,M}}_t,e^{\varepsilon}_m \rangle \langle    X^{u^{*,M}_t(z)}_t -X^{u^{*,M} }_t ,\Delta e^{\varepsilon }_m \bigr\rangle   \d t 
\\
		& +2\sum_{m\geq 0}\langle X_t^{u_t^{*,M}(z)}-X^{u^{*,M}}_t,e^{\varepsilon}_m \rangle \left(\d\bigl\langle \tilde{\eta}^{ u,(z,1)}_t, e^{\varepsilon}_m \bigr\rangle -\d\bigl\langle {\eta}_t, e^{\varepsilon}_m \bigr\rangle  \right) 
		\nonumber	
		\\
		& -  \tfrac{2}{T} \sum_{m\geq 0}\langle X_t^{u_t^{*,M}(z)}-X^{u^{*,M}}_t,e^{\varepsilon}_m \rangle {\times \bigl( }   \partial_y \bigl\langle  X^{u^{*,M}_t(z)}_t ,e^\varepsilon_m\bigr\rangle \cdot z   {\bigr)}  \,   \d t
		\nonumber	
		\\
		= :& S_1+S_2+S_3. \label{eq itoLipShift}
	\end{align}
\emph{Handling} $S_1$: One uses the self-adjoint property of $e^{\varepsilon\Delta}$, followed by Parseval's theorem and integration by parts to obtain: $$2\sum_{m\geq 0}\langle X_t^{u_t^{*,M}(z)}-X^{u^{*,M}}_t,e^{\varepsilon}_m \rangle \langle    X^{u^{*,M}_t(z)}_t -X^{u^{*,M} }_t ,\Delta e^{\varepsilon }_m \bigr\rangle   = -2\lVert e^{\varepsilon\Delta} \nabla_x(X_t^{u_t^{*,M}(z)}-X^{u^{*,M}}_t)\rVert_2^2.$$
\emph{Handling} $S_2$: This expression has non-positive limit inferior as $\varepsilon$ tends to zero. This follows by Corollary 4.8 in \cite{delarueHammersley2022rshe} and the fact that the minimality condition \eqref{def RSHE 2} may be strengthened to an almost sure statement via the argument following Proposition 4.11 in \cite{delarueHammersley2022rshe}, namely that $\bP$ almost surely
\begin{equation}
	\notag 
	\liminf_{\varepsilon\searrow0} \int_0^t  \langle e^{\varepsilon\Delta}X_r  , \d  \eta_r \rangle= 0.
\end{equation}
Consequently, the analogous statement for the shifted process and its tilted reflection process holds on the equivalent probability space $\bQ$ and hence also on $\bP$. To explicit, $\bQ$ and $\bP$ almost surely,
\begin{equation}
	\notag 
	\liminf_{\varepsilon\searrow0} \int_0^t \langle  e^{\varepsilon\Delta} X_r^{x_r^{*,M}(z)}  , \d  \tilde{\eta}^{ x,(z,1)}_r \rangle= 0.
\end{equation}
\emph{Handling} $S_3$: Naturally, for the {penultimate} line in \eqref{eq itoLipShift}, it is tempting to rewrite this as a derivative in $E^M$ of $\langle X_t^{u_t^{*,M}(z)}-X^{u^{*,M}}_t,e^{\varepsilon}_m \rangle^2$ and dismiss the term due to a negative sign. However, the presence of the rearrangement in the superscript poses a technical barrier. Fortunately, in the present setting one does not require such a fine estimate and can brutally estimate with Young's inequality. 
\begin{equation}
	\begin{split} 
		& -  \tfrac{2}{T} \sum_{m\geq 0}\langle X_t^{u_t^{*,M}(z)}-X^{u^{*,M}}_t,e^{\varepsilon}_m \rangle {\times \bigl( }   \partial_y \bigl\langle  X^{u^{*,M}_t(z)}_t ,e^\varepsilon_m\bigr\rangle \cdot z  {\bigr)} 
		\\
		&\leq     \bigl\lVert e^{\varepsilon\Delta}(X_t^{u_t^{*,M}(z)}-X^{u^{*,M}}_t) \bigr\rVert_2^2 + \tfrac{1}{T^2} \sum_{m\geq 0} |  \partial_y \bigl\langle  X^{u^{*,M}_t(z)}_t ,e^\varepsilon_m\bigr\rangle \cdot z |^2  \\
	\end{split}
\end{equation}
Returning to \eqref{eq itoLipShift}, applying the above inequality and the limit inferior as $\varepsilon\searrow 0 $ {yields the claim}.
 \end{proof}

Consider introducing a linear drifted to the rearranged stochastic heat equation:
\begin{equation}
\label{eq:RSHE:reverting:lambda} 
\d  X_t^{\mu} = - \mu X_t^{\mu} \d t + \Delta X_t^{\mu} \d t + \d W_t + \d \eta_t
\end{equation}
for a parameter $\mu >0$. The flow generated by \eqref{eq:RSHE:reverting:lambda}, started from $u\in U^2(\mathbb{S})$ is denoted 
$(X_t^{\mu,u},\eta_t^{\mu,u})_{t \geq 0}$. 
We refer to \eqref{eq:RSHE:reverting:lambda}
as the \textit{linearly} drifted 
RSHE (as opposed to the $F$-drifted equation
introduced in Definition 
\ref{def:existence}). 

There is no difficulty in proving the following 
variant of Proposition 4.18 in 
\cite{delarueHammersley2022rshe}. 

\begin{lemma}
\label{lem:reg:OU:RSHE}
For any $u,v \in U^2({\mathbb S})$, 
with probability 1,
for all $t \geq 0$, 
\begin{equation*} 
\| X_t^{\mu,u} - X_t^{\mu,v} \|_2^2 \leq \exp \bigl( - 2\mu t \bigr) 
\| u -v \|_2^2, 
\end{equation*}
\begin{equation*}
\int_0^t 
\| \nabla_x\left(X_s^{\mu,u} - X_s^{\mu,v} \right)\|_2^2 \d s \leq %\exp \bigl( - \mu t \bigr) 
\frac{1}{2 } \| u -v \|_2^2, 
\end{equation*}  
and
\begin{equation*}
\int_0^t 
\| X_s^{\mu,u} - X_s^{\mu,v} \|_2^2 \d s \leq %\exp \bigl( - \mu t \bigr) 
\frac{1}{2\mu} \| u -v \|_2^2, 
\end{equation*}

\end{lemma} 

\begin{proof}
We just provide a sketch of the proof. Following 
the proof of Proposition 4.18 in 
\cite{delarueHammersley2022rshe}, we have, for all $s,t \geq 0$, 
\begin{equation*}
\begin{split}
&\| X_t^{\mu,u} - X_t^{\mu,v} \|_2^2+ 2 \int_s^t \bigl\| \nabla_x \bigl( X_r^{\mu,u} - X_r^{\mu,v} \bigr) 
\bigr\|_2^2 \d r + 2 \mu \int_s^t \|   X_r^{\mu,u} -   X_r^{\mu,v} \|_2^2 
\d r 
\\
&\leq \| X_s^{\mu,u} - X_s^{\mu,v} \|_2^2,
\end{split}
\end{equation*} 
from which the result easily follows. 
\end{proof}

This lemma, in combination with Theorem 5.11 in \cite{delarueHammersley2022rshe}, yields the following: 
\begin{proposition}
\label{prop:5:5:rev}
There exists a constant $c$ such that, for any $\delta>0$, $T>\delta$ and any $u,v \in U^2({\mathbb S})$,  
\begin{equation*} 
d_{\rm TV} \bigl( {\mathscr L}(X_T^{\mu,u}) , {\mathscr L}(X_T^{\mu,v}) \bigr) \leq 
c_\lambda \delta^{-\frac{1+\lambda}{2}}
\exp\bigl( -  \mu (T-\delta ) \bigr)
 \| u - v \|_2, 
 \end{equation*} 
where the left-hand side denotes the total variation distance between 
${\mathscr L}(X_T^{\mu,u})$ and 
${\mathscr L}(X_T^{\mu,v})$, probability measures on 
$U^2({\mathbb S})$. 
\end{proposition} 

\begin{proof} 
We introduce the useful notation 
\begin{equation*} 
P_t^\mu \varphi(u) := {\mathbb E} \bigl[ \varphi(X_t^{\mu,u}) \bigr], \quad u \in U^2({\mathbb S}), 
\end{equation*} 
for $\varphi \in B_b(L^2_{sym}({\mathbb S}))$. 
Then, for $T>\delta$,
\begin{equation*} 
P^\mu_{T} \varphi(u) - P^\mu_{T} \varphi(v)
= {\mathbb E} \bigl[ P_\delta^{\mu} \varphi  (X_{T-\delta}^{\mu,u}) 
\bigr] - 
{\mathbb E} \bigl[ P_\delta^{\mu} \varphi  (X_{T-\delta}^{\mu,v} ) \bigr]
\end{equation*} 
There is no difficulty in adapting the main Theorem 5.11 from \cite{delarueHammersley2022rshe} to this \emph{linearly drifted} setting, proving that 
the function $P_\delta^\mu \varphi$ is Lipschitz continuous, with a Lipschitz constant bounded by 
$c_\lambda \delta^{-\frac{1+\lambda}{2}} \| \varphi\|_\infty$, with $c_\lambda$  independent of $\mu \in (0,+\infty)$ (which follows from the fact that the regularity of the flow, as stated in 
Lemma \ref{lem:reg:OU:RSHE}, is independent of $\mu$). 
And then,
\begin{equation*} 
\begin{split} 
\bigl\vert P^\mu_{T} \varphi(u) - P^\mu_{T} \varphi(v) \bigr\vert 
&\leq c_{\lambda} \delta^{-\frac{1+\lambda}{2}} \| \varphi \|_\infty {\mathbb E} \bigl[ \| X_T^{\mu,u} - X_T^{\mu,v} \|_2 \bigr] \\
 & \leq c_{\lambda} \delta^{-\frac{1+\lambda}{2}} \exp \bigl( - \mu T \bigr) \|\varphi \|_\infty  \| u - v \|_2,
\end{split}
\end{equation*}
with the last line following from 
Lemma 
\ref{lem:reg:OU:RSHE}.
\end{proof}

We return to the study of the RSHE drifted by $F$. For any fixed $T>0$, we can rewrite the equation solved by (the \emph{linearly drifted})
$X^{\mu,u}$
as
\begin{equation*}
\begin{split} 
\d X_t^{\mu,u} &= \Bigl( F(X_t^{\mu,u}) {\mathbf 1}_{\{ t \le T\}}
- \mu X_t^{\mu,u} {\mathbf 1}_{\{ t >T\}} 
\Bigr)
\d t 
\\
&\hspace{15pt} + \Delta X_t^{\mu,u} \d t +  \Bigl[\d W_t - 
\bigl(  F(X_t^{\mu,u}) + \mu X_t^{\mu,u}   \bigr) {\mathbf 1}_{\{ t \le T\}} \d t \Bigr] + \d \eta_t^{\mu,u}, \quad t \geq 0,
\end{split} 
\end{equation*}  
and define
\begin{equation} 
\label{eq:PT:F,x}
{\mathbb P}_T^{F,u} :=
{\mathcal E}_T \biggl\{ \int_0^{\cdot} \sum_{m \in {\mathbb N}_0} \lambda_m^{-1}
\bigl\langle F(X_t^{\mu,u}) + \mu X_t^{\mu,u}   , e_m \bigr\rangle \d \beta_s^{m} 
\biggr\} \cdot {\mathbb P} .
\end{equation} 
By an easy adaptation of Lemma \ref{lem:PF:P}, 
${\mathbb P}_T^{F,u}$ is a probability measure. Furthermore, under ${\mathbb P}_T^{F,u}$, 
$(X_t^{\mu,u})_{0 \le t \le T}$ solves the $F$-drifted RSHE  on the interval 
$[0,T]$ with $u$ as initial condition, and 
$(X_t^{\mu,u})_{t \geq T}$ solves the linearly drifted RSHE on $[T,+\infty)$ with $X_T^{\mu,u}$ as initial condition at time $T$.

We claim 
%(recalling that $\| u \|_2 \leq R):$
\begin{lemma} 
\label{lem:dTV:by:entropy}
Let $\delta>0$ $($be a small time duration in $(0,1))$, and $u\in U^2(\mathbb{S})$ be such that 
$\| u \|_2 \leq R$. Then, there exists a constant $C_{col,F,\lambda,R}$ (independent of $\mu$, $\delta$, and $T$) such that
\begin{equation*} 
d_{\rm TV} \bigl(  {\mathbb P}^{F,u}_T  ,
 {\mathbb P}_{T+\delta}^{F,u}
 \bigr) \leq  C_{col,F,\lambda,R} \cdot \mu \delta^{\frac{1-\lambda}{2}},
 \end{equation*} 
 with $\lambda$ as in \eqref{eq colouring}.
\end{lemma}
\begin{proof} 
The proof relies on the computation of the relative entropy 
\begin{equation*} 
\begin{split} 
{\mathbb E}^{ {\mathbb P}^{F,u}_{T}} \Bigl[ - \ln \Bigl( \frac{ \d {\mathbb P}^{F,u}_{T+\delta}}{\d {\mathbb P}^{F,u}_{T}} \Bigr) 
\Bigr].
\end{split}
\end{equation*}
Here, 
\begin{equation*} 
\begin{split}
\ln \Bigl( \frac{ \d {\mathbb P}^{F,u}_{T+\delta}}{\d {\mathbb P}^{F,u}_{T}} \Bigr)
&=
\sum_{m \in {\mathbb N}_0} \int_{T}^{T+\delta} 
  \lambda_m^{-1}
\bigl\langle  F(X_t^{\mu,u}) + \mu X_t^{\mu,u} , e_m \bigr\rangle \d \beta_s^{m} 
\\
&\hspace{15pt} - 
\frac12 
\sum_{m \in {\mathbb N}_0} \int_{T}^{T+\delta} 
  \lambda_m^{-2}
\bigl\vert \bigl\langle  F(X_t^{\mu,u}) + \mu X_t^{\mu,u} , e_m \bigr\rangle
\bigr\vert^2
 \d t.
 \end{split} 
\end{equation*} 
And then, 
\begin{equation*} 
{\mathbb E}^{ {\mathbb P}^{F,u}_{T}} \Bigl[ - \ln \Bigl( \frac{ \d {\mathbb P}^{F,u}_{T+\delta}}{\d {\mathbb P}^{F,u}_{T}} \Bigr) 
\Bigr]
= 
\frac12 
{\mathbb E}^{ {\mathbb P}^{F,u}_{T}} \biggl[
\sum_{m \in {\mathbb N}_0} \int_{T}^{T+\delta} 
  \lambda_m^{-2}
\bigl\vert \bigl\langle  F(X_t^{\mu,u}) + \mu X_t^{\mu,u} , e_m \bigr\rangle
\bigr\vert^2
 \d t
\biggr]. 
\end{equation*} 
To estimate the above, we proceed as follows. \textcolor{orange}{Need to be careful of low modes}
\begin{equation} 
\label{eq:mu:F:HSPLIT}
\begin{split} 
&\sum_{m \in {\mathbb N}_0} \int_{T}^{T+\delta} 
  \lambda_m^{-2}
\bigl\vert \bigl\langle  F(X_t^{\mu,u}) + \mu X_t^{\mu,u} , e_m \bigr\rangle
\bigr\vert^2
 \d t 
\\
&  \int_{T}^{T+\delta}  \left( \sum_{m\leq M}+\sum_{m>M}\right)
  \lambda_m^{-2}
\bigl\vert \bigl\langle  F(X_t^{\mu,u}) + \mu X_t^{\mu,u} , e_m \bigr\rangle
\bigr\vert^2
 \d  t
\\
&\leq     \int_{T}^{T+\delta} {\max_{m=1,\cdots,M} \lambda_m^{-2}}  \lVert F(X_t^{\mu,u}) + \mu X_t^{\mu,u} \rVert_2^2  
	+	  \sum_{m>M} \lambda_m^{-2}
\bigl\vert \bigl\langle  F(X_t^{\mu,u}) + \mu X_t^{\mu,u} , e_m \bigr\rangle
\bigr\vert^2  
 \d t
 \\		
\end{split} 
\end{equation}  
Next, by H\"older's inequality, 
\textcolor{red}{should change the notation $x$ for the starting point as there is a confusion 
with $\nabla_x$} \textcolor{orange}{Changed $x,y$ to $u,v$. Also, there is a constant prefactor coming from the fact that $\lambda_m$ is not defined so precisely in this paper - just its tail behaviour.}
\begin{equation} 
\label{eq:mu:F:Holder}
\begin{split} 
&{\mathbb E}^{ {\mathbb P}^{F,u}_{T}} \sum_{m >M} \int_{T}^{T+\delta} 
  \lambda_m^{-2}
\bigl\vert \bigl\langle  F(X_t^{\mu,u}) + \mu X_t^{\mu,u} , e_m \bigr\rangle
\bigr\vert^2
 \d s
\\
& \leq C_{col} {\mathbb E}^{ {\mathbb P}^{F,u}_{T}}
\sum_{m \in {\mathbb N}} \int_{T}^{T+\delta} 
   m^{2 \lambda}
\bigl\vert \bigl\langle  F(X_t^{\mu,u}) + \mu X_t^{\mu,u} , e_m \bigr\rangle
\bigr\vert^2
 \d s
 \\
 &\leq C_{col}\biggl( {\mathbb E}^{ {\mathbb P}^{F,u}_{T}}\sum_{m \in {\mathbb N}} \int_{T}^{T+\delta} 
  m^2
\bigl\vert \bigl\langle  F(X_t^{\mu,u}) + \mu  X_t^{\mu,u} , e_m \bigr\rangle
\bigr\vert^2
 \d s \biggr)^\lambda 
 \\
&\hspace{15pt} \times \biggl( {\mathbb E}^{ {\mathbb P}^{F,u}_{T}}\sum_{m \in {\mathbb N}} \int_{T}^{T+\delta} 
\bigl\vert \bigl\langle  F(X_t^{\mu,u}) + \mu  X_t^{\mu,u} , e_m \bigr\rangle
\bigr\vert^2
 \d s \biggr)^{1-\lambda}
 \\
 & \leq C_{col} \biggl( {\mathbb E}^{ {\mathbb P}^{F,u}_{T}}\int_T^{T+\delta} \bigl\| \nabla_x \bigl( F(X_t^{\mu,u}) + \mu X_t^{\mu,u} 
 \bigr) \bigr\|_2^2 \d s
 \biggr)^\lambda
 \times \biggl( {\mathbb E}^{ {\mathbb P}^{F,u}_{T}} \int_{T}^{T+\delta} 
\bigl\| F(X_t^{\mu,u}) + \mu  X_t^{\mu,u} 
\bigr\|_2^2
 \d s \biggr)^{1-\lambda}.
\end{split} 
\end{equation}  
%Next, by Assumption 
%\ref{ass drift eu}, 
%\begin{equation*} 
%\begin{split} 
%& {\mathbb E}^{ {\mathbb P}^{F,u}_{T}} \sum_{m \in {\mathbb N}_0} \int_{T}^{T+\delta} 
%  \lambda_m^{-2}
%\bigl\vert \bigl\langle  F(X_t^{\mu,u}) +  \mu X_t^{\mu,u} , e_m \bigr\rangle
%\bigr\vert^2
% \d s
% \\
% &\leq C_{col,F} \cdot \mu^2 
% \left( \delta + \int_T^{T+\delta}\bigl\|  X_t^{\mu,u} 
%\bigr\|_2^2 \d t   + 
% \biggl( \int_T^{T+\delta} \| \nabla_x X_t^{\mu,u} \|_2^2 \d 
% t \biggr)^{\lambda} 
% \biggl( \int_T^{T+\delta} \| X_t^{\mu,u} \|_2^2 \d 
% t 
%\biggr)^{1-\lambda}
%\right). 
%\end{split} 
%\end{equation*} 
And then, 
using the fact that, under ${\mathbb P}^{F,u}_T$, the process $(X_s^{\mu,u})_{T \leq s \leq T+\delta}$ 
solves the linearly drifted RSHE, with $X_T^{\mu,u}$ as initial condition,  
and
following the derivation of Proposition \ref{prop ito fsquare}, 
\begin{equation*} 
{\mathbb E}^{{\mathbb P}_T^{F,u}} \biggl[ \int_T^{T+\delta} \| \nabla_x X_t^{\mu,u} \|_2^2 \d 
 t \, \Bigr\vert \, {\mathcal F}_T \biggr] \leq \| X_T^{\mu,u} \|^2_2 + c_\lambda \delta,
 \end{equation*} 
 and 
 \begin{equation*} 
\sup_{T \le t \le T +\delta} 
 {\mathbb E}^{{\mathbb P}_T^{F,u}} \bigl[ 
 \| X_t^{\mu,u} \|_2^2 \, \bigr\vert \, {\mathcal F}_T
 \bigr]
 \leq   \| X_T^{\mu,u} \|^2_2 + c_\lambda \delta,
 \end{equation*} 
Therefore, from Assumption \ref{ass drift eu}, 
\begin{equation*} 
\begin{split}
{\mathbb E}^{{\mathbb P}_T^{F,u}} \biggl[ 
\sum_{m \in {\mathbb N}_0} \int_{T}^{T+\delta} 
  \lambda_m^{-2}
\bigl\vert \bigl\langle  F(X_t^{\mu,u}) + \mu X_t^{\mu,u} , e_m \bigr\rangle
\bigr\vert^2
 \d t \, \Bigr\vert \, {\mathcal F}_T \biggr]
 &\leq C_{col,F,\lambda}\cdot\mu^2 \delta^{1-\lambda} \Bigl( 1+ \| X_T^{\mu,u} \|^2_2 \Bigr). 
 \end{split}
 \end{equation*} 
We deduce that 
\begin{equation*}
\begin{split} 
&{\mathbb E}^{ {\mathbb P}^{F,u}_{T}} \Bigl[ - \ln \Bigl( \frac{ \d {\mathbb P}^{F,u}_{T+\delta}}{\d {\mathbb P}^{F,u}_{T}} \Bigr) 
\Bigr]
\leq C_{col,F,\lambda}\cdot\mu^2 \delta^{1-\lambda}  \bigl( 1 +  {\mathbb E}^{{\mathbb P}^{F,u}_{T}}  \bigl[ \vert X_T^{\mu,u} \vert^2 \bigr] \bigr), 
 \end{split}
\end{equation*} 
where we observe that the moment appearing in the right-hand side is nothing but the second-order moment 
of the $F$-drifted  
RSHE starting from $u$, which can be bounded independently of $T$ and $u$ (as long as $\| u \|_2 \leq R$). For a proof of this latter assertion, one may refer to \eqref{eq unifEstBall 6}. \textcolor{red}{should we provide a proof for this?} In other words, the rightmost factor in the above may be bounded by a constant $C_R$.

By the Bretagnolle-Huber inequality \textcolor{red}{the original article by Bretagnolle and Huber is rather difficult to read, it might be more convenient to cite the slightly weaker inequality obtained in the book by Tsybakov that I put in the dropbox (see page 88 in the book)}, we get
\begin{equation*} 
d_{\rm TV} \bigl(  {\mathbb P}^{F,u}_T  ,
 {\mathbb P}_{T+\delta}^{F,u}
 \bigr) \leq 
\sqrt{1 - e^{- C_{col,F,\lambda,R} \cdot \mu^2 \delta^{1-\lambda}  }}.
\end{equation*} 
 The result easily follows, recalling that the value of the constant may change.
\end{proof}

% and 
%\begin{equation*} 
%\begin{split} 
%{\mathbb E} \Bigl[ - \ln \Bigl( \frac{ \d {\mathbb P}^{F,x}}{d {\mathbb P}} \Bigr) 
%\Bigr] 
%= \frac12 {\mathbb E} \biggl[ 
%\int_0^{\cdot} \sum_{m \in {\mathbb N}_0} \mu_m^{-1}
%\bigl\vert  \bigl\langle F(X_t^{\mu,u}) - \mu X_t^{\mu,u} , e_m \bigr\vert^2 \biggr]. 
% \end{split}
% \end{equation*} 
 
We now consider another initial condition $v \in U^2({\mathbb S})$. We recall that 
\begin{equation*} 
\d X_t^{\mu,v} = \mu X_t^{\mu,v} \d t + \Delta X_t^{\mu,v} \d t  + 
\d W_t
%\bigl[ \d W_t + \bigl( \mu X_t^{\mu,u}
%-F(X_t^{\mu,u})  \bigr) {\mathbf 1}_{\{ t \le T\}} \d t \bigr] 
+ 
\d \eta_t^{\mu,v}, \quad t \geq 0.
\end{equation*} 
We claim  
\begin{lemma}
\label{lem:DKL:1}
There exists a constant $C_{col,F,\lambda,R}$ $($independent of $\delta$, $T$, and $\mu)$ such that, for $\| u \|_2,\| v \|_2 \leq R$, 
 \begin{equation*} 
d_{\rm TV} \bigl( {\mathscr L}_{{\mathbb P}_{T+\delta}^{F,u}}(X_{T+\delta}^{\mu,u}) , {\mathscr L}_{{\mathbb P}_{T+\delta}^{F,u}}(X_{T+\delta}^{\mu,v}) \bigr) \leq  C_{col,F,\lambda,R} \left(\delta^{-\frac{1+\lambda}{2}}\exp\bigl( - \mu (T-\delta) \bigr) + \mu \delta^{\frac{1-\lambda}{2}} \right)   
 \end{equation*}
\end{lemma}

\begin{proof}
For a test function $\varphi$ as in the proof of Proposition 
\ref{prop:5:5:rev} and a real $\delta >0$, 
we compute
\begin{equation*}
\begin{split} 
&{\mathbb E}^{{\mathbb P}_T^{F,u}} \bigl[ \varphi\bigl(X_{T+\delta}^{\mu,v}\bigr) \bigr]
- 
{\mathbb E}^{{\mathbb P}_T^{F,u}} \bigl[ \varphi\bigl(X_{T+\delta}^{\mu,u}\bigr) \bigr]
 ={\mathbb E}^{{\mathbb P}_T^{F,u}} \Bigl[  {\mathbb E}^{{\mathbb P}_T^{F,u}}
\bigl[ \varphi\bigl(X_{T+\delta}^{\mu,v}\bigr)  
- 
 \varphi\bigl(X_{T+\delta}^{\mu,u}\bigr) \vert {\mathcal F}_T \bigr] \Bigr].
\end{split} 
\end{equation*} 
Since $\d {\mathbb P}_T^{F,u}/\d {\mathbb P}$ is ${\mathcal F}_T$-measurable, 
we have  
\begin{equation*}
  {\mathbb E}^{{\mathbb P}_T^{F,u}}
\bigl[ \varphi\bigl(X_{T+\delta}^{\mu,v}\bigr)  
- 
 \varphi\bigl(X_{T+\delta}^{\mu,u}\bigr) \vert {\mathcal F}_T \bigr]
 = P_\delta^\mu \varphi \bigl( X_T^{\mu,v} \bigr) 
 - P_\delta^\mu \varphi\bigl( X_T^{\mu,u} \bigr),
 \end{equation*}
 where 
 $(P_t^{\mu})_{t \geq 0}$ denotes the semi-group generated by 
 the linearly drifted RSHE, see 
the proof of 
Proposition \ref{prop:5:5:rev}. 
In particular, the result of Proposition 
 \ref{prop:5:5:rev} remains true under 
${\mathbb P}_T^{F,x}$, for times after $T$, namely
% \begin{equation*} 
%d_{\rm TV} \bigl( {\mathscr L}_{{\mathbb P}^{F,x}}(X_{T+1}^{\mu,u}) , {\mathscr L}_{{\mathbb P}^{F,x}}(X_{T+1}^{\mu,v}) \bigr) \leq 
%c
%\exp\bigl( - \mu (T-1) \bigr)
% \| x - y \|_2, 
% \end{equation*} 
% In fact, we can change this result into 
 \begin{equation*} 
d_{\rm TV} \bigl( {\mathscr L}_{{\mathbb P}_T^{F,u}}(X_{T+\delta}^{\mu,u}) , {\mathscr L}_{{\mathbb P}_T^{F,u}}(X_{T+\delta}^{\mu,v}) \bigr) \leq 
\frac{c_\lambda}{\delta^{(1+\lambda)/2}} 
\exp\bigl( -  \mu (T-\delta) \bigr)
 \| u - v \|_2, 
 \end{equation*}  
Then, by Lemma 
\ref{lem:dTV:by:entropy}, 
 \begin{equation*} 
d_{\rm TV} \bigl( {\mathscr L}_{{\mathbb P}_{T+\delta}^{F,u}}(X_{T+\delta}^{\mu,u}) , {\mathscr L}_{{\mathbb P}_{T+\delta}^{F,u}}(X_{T+\delta}^{\mu,v}) \bigr) \leq 
\frac{c_\lambda}{\delta{(1+\lambda)/2}} 
\exp\bigl( - \mu (T-\delta) \bigr)
 \| u - v \|_2 + 2 \cdot C_{col,F,\lambda,R} \cdot \mu \delta^{\frac{1-\lambda}{2}}  
 \end{equation*} 
 This completes the proof, recalling that $u,v$ have $L^2$ norm bounded by $R$. 
 \end{proof}

 \begin{lemma}
\label{lem:DKL:2}
There exist a constant $C_{\mu,R}$, only depending on $\mu$ and $R$ (together with the constants in the assumptions on $F$), and a constant $C_R$, only depending on $R$ (together with the constants in the assumptions on $F$), such that 
\begin{equation*} 
d_{\rm TV} \bigl( {\mathscr L}_{{\mathbb P}_{T+\delta}^{F,u}}(X_{T+\delta}^{\mu,v}) , {\mathscr L}_{{\mathbb P}_{T+\delta}^{F,v}}(X_{T+\delta}^{\mu,v}) \bigr) \leq  
\sqrt{1 - \exp \bigl( - C_{col,F,\lambda,R} ( (T+\delta) + C_\mu )
\bigr)}.
\end{equation*} 
\end{lemma} 
\begin{proof}
 We compute
 the relative entropy of 
 ${\mathbb P}_{T+\delta}^{F,v}$
 with respect to 
 ${\mathbb P}_{T+\delta}^{F,u}$. Using 
 the expression of each of the two densities, see 
  \eqref{eq:RSHE:reverting:lambda} , we obtain 
 \begin{equation}
\label{eq:dTB:last:step:mu:-1}
 \begin{split}
& {\mathbb E}^{{\mathbb P}_{T+\delta}^{F,u}}
 \Bigl[ - 
 \ln \Bigl( \frac{\d {\mathbb P}_{T+\delta}^{F,v}}{\d {\mathbb P}_{T+\delta}^{F,u}}
 \Bigr)\Bigr]
 \\
 &\hspace{5pt} =
 \frac12
 {\mathbb E}^{{\mathbb P}_{T+\delta}^{F,u}}
 \biggl[ 
 \int_0^{T+\delta}  \sum_{m \in {\mathbb N}_0} \lambda_m^{-2}
\bigl\langle  F(X_t^{\mu,u}) - F(X_t^{\mu,v}) + \mu (X_t^{\mu,u} - X_t^{\mu,v}), e_m \bigr\rangle^2
\d t
\biggr].
\end{split} 
\end{equation} 
Proceeding as in \eqref{eq:mu:F:HSPLIT} and \eqref{eq:mu:F:Holder}, we have
\begin{equation} 
\label{eq:dTB:last:step:mu:0}
\begin{split}
& {\mathbb E}^{{\mathbb P}_{T+\delta}^{F,u}} \int_0^{T+\delta}  \sum_{m \in {\mathbb N}_0} \mu_m^{-2}
\bigl\langle  F(X_t^{\mu,u}) - F(X_t^{\mu,v}) + \mu (X_t^{\mu,u} - X_t^{\mu,v}), e_m \bigr\rangle^2
 \d t
\\
&\leq C_{col}   
 \bigg(  
  {\mathbb E}^{{\mathbb P}_{T+\delta}^{F,u}}
 \int_0^{T+\delta} 
\bigl\| 
F(X_t^{\mu,u}) - F(X_t^{\mu,v}) +  \mu (X_t^{\mu,u} - X_t^{\mu,v})
\bigr\|_2^2 \d t \\
&   + 
 \biggl( 
  {\mathbb E}^{{\mathbb P}_{T+\delta}^{F,u}}
  \int_0^{T+\delta} 
\bigl\| \nabla_x 
\bigl( 
F(X_t^{\mu,u}) - F(X_t^{\mu,v}) +  \mu (X_t^{\mu,u} - X_t^{\mu,v}) \bigr) 
\bigr\|_2^2 \d t  \biggr)^{\lambda} \\
\cdot & 
 \biggl(
  {\mathbb E}^{{\mathbb P}_{T+\delta}^{F,u}}
   \int_0^{T+\delta} 
\bigl\| 
F(X_t^{\mu,u}) - F(X_t^{\mu,v}) +\mu (X_t^{\mu,u} - X_t^{\mu,v}) 
\bigr\|_2^2 \d t
\biggr)^{1-\lambda}.
\end{split}
\end{equation}
 By Lemma 
 \ref{lem:reg:OU:RSHE}, we obtain 
 \begin{equation}
 \label{eq:dTB:last:step:mu:1}
\begin{split}
&\int_0^{T+\delta}   \bigl\|   \nabla_x   \bigl(X_t^{\mu,u} - X_t^{\mu,v} \bigr) 
\bigr\|_2^2 
\d t \leq 4 R^2, 
\\
&\mu ^2 \int_0^{T+\delta}   \|   X_t^{\mu,u} - X_t^{\mu,v}  
\|_2^2 
\d t
%\leq 4 R^2 \int_0^{T+\delta}  \exp(- \mu s ) ds
 \leq 4\mu R^2
\end{split}
\end{equation}
By Assumption 
\ref{ass drift bounded oscillation} and by Lemma  \ref{lem:reg:OU:RSHE}, 
\begin{equation} 
\label{eq:dTB:last:step:mu:2}
\int_0^{T+\delta}  \| F(X_t^{\mu,u}) - F(X_t^{\mu,v})\|_2^2 \d t
\leq (T+\delta) \bigl( C_O(2R) \bigr)^2.  
\end{equation} 
Next,
by Assumption \ref{ass drift eu} and \eqref{eq:dTB:last:step:mu:1}, 
\begin{equation} 
\label{eq:dTB:last:step:mu:3}
\begin{split}
\int_0^{T+\delta}  \bigl\| \nabla_x \bigl(  F(X_t^{\mu,u}) - F(X_t^{\mu,v}) \bigr) \bigr\|_2^2 \d t
&\leq C_F  
\int_0^{T+\delta} \Bigl(  \bigl\| \nabla_x X_t^{\mu,u} \bigr\|_2^2 + 
\bigl\| \nabla_x X_t^{\mu,v} \bigr\|_2^2
\Bigr)  \d t
\\
&\leq C_F\left( R^2 +   \int_0^{T+\delta}   \bigl\| \nabla_x X_t^{\mu,u} \bigr\|_2^2  \d t\right).
\end{split}
\end{equation} 
Following the derivation of  
Proposition \ref{prop zeroMode} \textcolor{red}{could be made more explicit}, we 
have
$$ {\mathbb E}^{{\mathbb P}_{T+\delta}^{F,x}}\int_0^{T+\delta}   \bigl\| \nabla_x X_t^{\mu,u} \bigr\|_2^2  \d t
\leq C_\lambda(  R^2+ (T+\delta)).$$
Collecting 
\eqref{eq:dTB:last:step:mu:-1},
\eqref{eq:dTB:last:step:mu:0},
\eqref{eq:dTB:last:step:mu:1},
\eqref{eq:dTB:last:step:mu:2}
and
\eqref{eq:dTB:last:step:mu:3}
\begin{equation*} 
\begin{split}
& {\mathbb E}^{{\mathbb P}_{T+\delta}^{F,x}}
 \Bigl[ - 
 \ln \Bigl( \frac{\d {\mathbb P}_{T+\delta}^{F,y}}{\d {\mathbb P}_{T+\delta}^{F,x}}
 \Bigr)\Bigr]
%\\
%&
 \leq C_{col,F,\lambda}  ( (C_O(2R)+R^2)(T+\delta) + C_R(1+\mu^2) )  
\\
%
%
%&\leq 
%\biggl(  {\mathbb E}^{{\mathbb P}_{T+\delta}^{F,x}}
%\int_0^{T+\delta} 
%\bigl\| \nabla_x 
%\bigl( 
%F(X_t^{\mu,u}) - F(X_t^{\mu,v}) - \mu (X_t^{\mu,u} - X_t^{\mu,v}) \bigr) 
%\bigr\|_2^2 \d t 
%\biggr)^\lambda(T+\delta)
%\\
%&\hspace{15pt} \times \biggl(  {\mathbb E}^{{\mathbb P}_{T+\delta}^{F,x}}
%\int_0^{T+\delta} 
%\bigl\| 
%F(X_t^{\mu,u}) - F(X_t^{\mu,v}) - \mu (X_t^{\mu,u} - X_t^{\mu,v}) 
%\bigr\|_2^2 \d t 
%\biggr)^{1-\lambda}
%\\
%&\leq C \Bigl(  c_\mu R^2 +  {\mathbb E}^{{\mathbb P}_{T+\delta}^{F,x}}\int_0^{T+\delta}   \bigl\| \nabla_x X_t^{\mu,u} \bigr\|_2^2  \d t
%\Bigr)^{\lambda} 
% \Bigl( c_\mu R^2 + C_R(T+\delta) 
%\Bigr)^{1-\lambda}, 
\end{split}
\end{equation*} 
%where $c_\mu$ only depends on $\mu$. 

%Finally, 
%\begin{equation*} 
%\begin{split}
%& {\mathbb E}^{{\mathbb P}_{T+\delta}^{F,x}}
% \Bigl[ - 
% \ln \Bigl( \frac{\d {\mathbb P}_{T+\delta}^{F,y}}{\d {\mathbb P}_{T+\delta}^{F,x}}
% \Bigr)\Bigr]
%\leq  C \Bigl(  c_\mu R^2 + C_R(T+\delta)
%\Bigr). 
%\end{split}
%\end{equation*} 
 The result follows by 
 Bretagnolle-Huber inequality. 
 \end{proof} 
 
 We now complete the proof
 of the coupling inequality 
\eqref{eq couplingEst}:
 \begin{proposition} 
Fix $R>0$ as before. Then, there exists a constant $C_{col,F,\lambda,R}$, such that for $(1-\lambda)\mu  > 8 C_{col,F,\lambda,R}$, we can find $c^*,T^*>0$, depending on $R,\mu,\lambda,C_{col}$ and the assumptions on $F$, yielding %only depending on $\mu$ and $R$ (and the assumptions on $F$)  
 \begin{equation*} 
  \begin{split} 
&d_{\rm TV} \bigl( {\mathscr L}_{{\mathbb P}_{T^*}^{F,u}}(X_{T**}^{\mu,u}) , {\mathscr L}_{{\mathbb P}_{T^*}^{F,v}}(X_{T^*}^{\mu,v}) \bigr) 
 \leq 1 - c^*. 
\end{split}  
 \end{equation*}
 \end{proposition} 
 
 \begin{proof}
 By expanding $\sqrt{1-r}$ for $r$ small, we can find a constant $c>0$ \textcolor{red}{should be $c=1/2$, and directly given by Tsybakov inequality} such that, 
 for $T$ sufficiently large, and $\delta$ sufficiently small, we deduce from Lemmas \ref{lem:DKL:1}
 and
\ref{lem:DKL:2} that
  \begin{equation*} 
  \begin{split} 
&d_{\rm TV} \bigl( {\mathscr L}_{{\mathbb P}_{T+\delta}^{F,x}}(X_{T+\delta}^{\mu,u}) , {\mathscr L}_{{\mathbb P}_{T+\delta}^{F,y}}(X_{T+\delta}^{\mu,v}) \bigr) 
\\
&\leq 
C_{col,F,\lambda,R} \left(\delta^{-\frac{1+\lambda}{2}}\exp\bigl( - \mu (T-\delta) \bigr) + \mu \delta^{\frac{1-\lambda}{2}} \right)   +\sqrt{1 - \exp \bigl( -C_{col,F,\lambda,R} ( (T+\delta) + C_\mu )
\bigr)}
\\
&\leq 1 + C_{col,F,\lambda,R} \left(\delta^{-1}\exp\bigl( - \mu (T-\delta) \bigr) + \mu \delta^{\frac{1-\lambda}{2}} \right)    - c \exp \bigl( - C_{col,F,\lambda,R} ( (T+\delta) + C_\mu )
\bigr).
\end{split}  
 \end{equation*}
Choosing $\delta = \exp(-\mu T/2)$ (with $T$ large so that $\delta \mu \leq 1$ and $\delta \le T/2$, which is doable -independently of $\mu$- if $\mu\geq 1$ for instance), we get 
 \begin{equation*} 
  \begin{split} 
&d_{\rm TV} \bigl( {\mathscr L}_{{\mathbb P}_{T+\delta}^{F,x}}(X_{T+\delta}^{\mu,u}) , {\mathscr L}_{{\mathbb P}_{T+\delta}^{F,y}}(X_{T+\delta}^{\mu,v}) \bigr) 
\\
&\leq 1 +  C_{col,F,\lambda,R} \Bigl[  
\exp\bigl(  - \mu T/4 \bigr)
+ \mu \exp \bigl( - \frac{(1-\lambda)\mu T}{4} \bigr) \Bigr]   - c \exp \bigl( - C_{col,F,\lambda,R} ( (T+\delta) + C_\mu )
\bigr)
\\
&= 1 + \exp \bigl( - 2 C_{col,F,\lambda,R} T \bigr) \Bigl[ C_{col,F,\lambda,R} \exp \bigl( (2 C_{col,F,\lambda,R} - \mu/4) T \bigr)
+ \exp \bigl( (2 C_{col,F,\lambda,R}  -\frac{(1-\lambda)\mu }{4} ) T \bigr)   
\\
&\hspace{15pt} - c \exp \bigl( - C_{col,F,\lambda,R}C_{\mu}   \bigr) 
\Bigr]. 
\end{split}  
 \end{equation*}
 Choosing $(1-\lambda)\mu  > 8 C_{col,F,\lambda,R}$, we see that the limit, as $T$ tends to $+\infty$, 
 of the term inside the bracket is negative. 
 \end{proof}
